# Supplementary material for: Negative piezoelectricity in low--dimensional materials
Source: arXiv:2009.10603 ancillary file (2021-04-20)
Supplement: Supplementary file 1 [file Supplemental_Materials.pdf]

# Supplementary Materials

Yubo Qi, and Andrew M. Rappe
Department of Chemistry,
University of Pennsylvania, Philadelphia, PA 19104-6323, United States

## I. METHODS

In this work, all DFT calculations are performed with the QUANTUM–ESPRESSO [S1] package, using optimized norm–conserving pseudopotentials generated by the OPIUM package [S2]. The electronic exchange–correlation energy is described by the generalized-gradient-approximation (GGA) density functional of Perdew, Burke, and Ernzerhof (PBE) [S3]. The plane–wave cutoff energy is set to 50 Ry. The force threshold for structural optimization is 10 meV/Å, and a 4×4×4 Monkhorst–Pack $k$–point mesh is used to sample the Brillouin zone [S4]. The vdW interaction is included via the DFT–D2 method [S5, S6] and the polarization is calculated by the Berry's phase method [S7].

## II. SCHEMATIC ILLUSTRATIONS OF THE CLAMPED–ION AND INTERNAL STRAIN TERMS

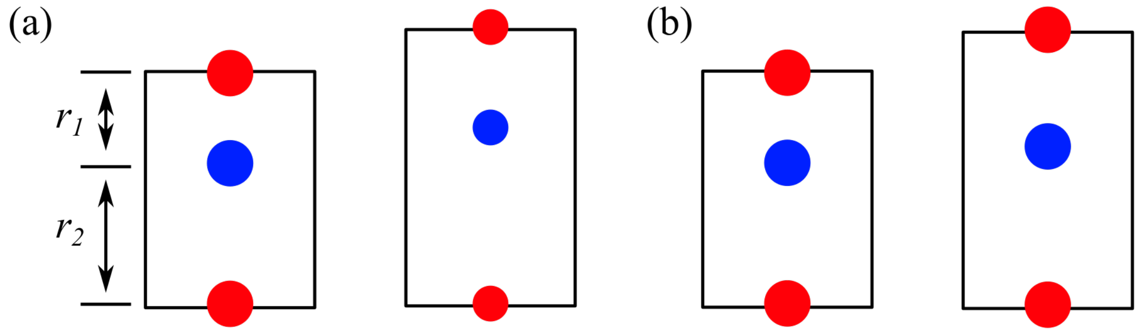


FIG. S1. Schematic illustrations of the (a) clamped–ion and (b) internal strain terms. The red and blue spheres represent cation and anion respectively. The sizes of the spheres represent the magnitudes of the Born effective charges.

The clamped–ion term describes the changes of the Born effective charges under a strain, assuming the internal fractional coordinates fixed. To evaluate this term, each chemical bond

are assumed to elongate homogeneously under a tensile strain, making the ratio between $r_1$ and $r_2$ remain the same [as shown in Fig. S1 (a)]. The magnitudes of the Born effective charges change due to the bond elongations.

The internal term describes the changes of the internal fractional coordinates under a strain, assuming the Born effective charges fixed. As reflected in Fig. S1 (b), the atoms locate at the optimized positions in different strained conditions. Therefore, the ratio between $r_1$ and $r_2$ may change. To evaluate the internal strain term, which describes the contribution from atomic distortion only, the magnitudes of the Born effective charges are assumed fixed.

## III. MAGNITUDES OF THE CLAMPED–ION TERM $e^{(0)}$ IN DIFFERENT MATERIALS

| Material | $e^{(0)}$ (C/m$^2$) | Material | $e^{(0)}$ (C/m$^2$) | Material | $e^{(0)}$ (C/m$^2$) |
|---|---|---|---|---|---|
| AlN[a] | −0.47 | BeO[a] | −0.60 | BeO[d] | −0.15 |
| GaN[a] | −0.84 | InN[a] | −0.88 | KMgAs[f] | −0.39 |
| LiBeAs[f] | −0.65 | LiBeBi[f] | −0.76 | LiBeP[f] | −0.63 |
| LiBeSb[f] | −0.70 | LiMgAs[f] | −0.12 | LiMgP[f] | −0.11 |
| LiZnAs[f] | −0.73 | LiZnP[f] | −0.62 | LiZnSb[f] | −0.95 |
| NaMgAs[f] | −0.26 | NaMgP[f] | −0.24 | NaMgSb[f] | −0.32 |
| NaZnSb[f] | −0.95 | $PbTiO_3$[c] | −0.88 | $PbTiO_3$[f] | −0.86 |
| $PbZr_{0.5}Ti_{0.5}O_3$[b] | −0.65 | $PbZr_{0.5}Ti_{0.5}O_3$[c] | −0.70 | $Sc_xAl_{1-x}N$[e] | −0.47∼−0.56 |
| ZnO[a] | −0.66 | ZnO[d] | −0.44 | ZnS[d] | −0.76 |

[a] Reference [S8]; [b] Reference [S9]; [c] Reference [S10]; [d] Reference [S11]; [e] Reference [S12]; [f] Reference [S13].

TABLE S1. The magnitudes of the clamped–ion terms reported in previous literatures. The materials are sorted with the alphabetical order. Some materials, such as ZnO, BeO and $PbTiO_3$, have different values of $e^{(0)}$. This mismatch can be attributed to the adoptions of different functionals.

## IV. DERIVATION OF THE EQUATION (7)

The Hamiltonian of a diatomic molecule is expressed as [S14]

$$\hat{H} = \hat{K}_e - \frac{1}{N}\sum_R \left[\frac{Z_A}{r_{iAR}} + \frac{Z_B}{r_{iBR}} + \frac{Z_A}{r_{jAR}} + \frac{Z_B}{r_{jBR}}\right] + \frac{1}{r_{ij}}, \tag{S1}$$

where $A$ and $B$ represent the atoms, $Z_A$ and $Z_B$ are the effective nuclear charges, and $i$ and $j$ correspond to the electrons. The term $\frac{Z_A}{r_{iAR}}$ describes the interaction between the electron $i$ and the nuclear $A$ in the unit cell locating at $R$.

Two electrons with the opposite spins occupy the valence band orbital, and we have

$$\Psi_k\left(r\right) = \psi_k\left(i, r\right)\psi_k\left(j, r\right). \tag{S2}$$

$$\psi_k\left(i, r\right) = \frac{1}{\sqrt{N}}\sum_R e^{ik\cdot R}\left[c_{A,k}\phi_A\left(i, r + R\right) + c_{B,k}\phi_B\left(i, r - d_1 + R\right)\right]. \tag{S3}$$

We assume that in a unit cell, atom $A$ locates at $R_A = 0$, atom $B$ locates at $R_B = d_1$, and the cell length is $d$. $R = nd$, where $n$ is an integer and runs from 1 to $N$.

In the hamiltonian matrix, we only consider the onsite integrals and the nearest-neighbor interactions. For the wavefunction overlaps, we only consider the onsite integrals. Other components are approximated as zero. Following the procedures in reference [S14], we decompose the energy

$$E_k = \langle\Psi_k|\hat{H}|\Psi_k\rangle \tag{S4}$$

into the following parts.

The kinetic energy term

$$\begin{aligned}\left\langle\Psi_k\left|-\frac{1}{2}\nabla_i^2 - \frac{1}{2}\nabla_j^2\right|\Psi_k\right\rangle &= 2(c_{A,k}^4 K_A + c_{A,k}^2 c_{B,k}^2 K_A + c_{B,k}^4 K_B + c_{A,k}^2 c_{B,k}^2 K_B) \\ &= 2(c_{A,k}^2 K_A + c_{B,k}^2 K_B)\end{aligned} \tag{S5}$$

where $K_{A(B)} = \langle\phi_{A(B)}(i, r)|-\frac{1}{2}\nabla_i^2|\phi_{A(B)}(i, r)\rangle$ is the kinetic energy of the electron on atomic orbital $\phi_{A(B)}$. Here, we approximate the terms $\langle\phi_A(i, r)|-\frac{1}{2}\nabla_i^2|\phi_A(i, r + R)\rangle$ $(R \neq 0)$ and $\langle\phi_A(i, r)|-\frac{1}{2}\nabla_i^2|\phi_B(i, r)\rangle$ as zero. We aslo use the normalization condition $c_{A,k}^2 + c_{B,k}^2 = 1$.

The core–electron interaction

$$
\begin{aligned}
&\left\langle \Psi_k \left| -\frac{1}{N} \sum_R \left[ \frac{Z_A}{r_{iAR}} + \frac{Z_B}{r_{iBR}} \right] \right| \Psi_k \right\rangle \\
=& - c_{A,k}^2 \left( \int \frac{\left|\phi_A(i,r)\right|^2 Z_A}{r_{iA}} d^3\tau_i + \int \frac{\left|\phi_A(i,r)\right|^2 Z_B}{r_{iB}} d^3\tau_i \right) \\
&- c_{B,k}^2 \left( \int \frac{\left|\phi_B(i,r-d_1)\right|^2 Z_B}{r_{iB}} d^3\tau_i + \int \frac{\left|\phi_B(i,r-d_1)\right|^2 Z_A}{r_{iA}} d^3\tau_i \right) \\
&- 2c_{A,k}c_{B,k} \int \phi_A(i,r) \left( \frac{Z_A}{r_{iA}} + \frac{Z_B}{r_{iB}} \right) \phi_B(i,r-d_1)\, d^3\tau_i \\
&- 2c_{A,k}c_{B,k} \cos k \int \phi_A(r) \left( \frac{Z_A}{r_{iA}} + \frac{Z_B}{r_{iB}+d} \right) \phi_B(i,r-d_1+d)\, d^3\tau_i \\
=& - c_{A,k}^2 \left(E_A + \Gamma_{Ba}\right) - c_{B,k}^2 \left(E_B + \Gamma_{Ab}\right) - 2c_{A,k}c_{B,k}\Gamma_{AB} - 2c_{A,k}c_{B,k} \cos k \Gamma_{AB}^*
\end{aligned}
\tag{S6}
$$

Here,

$$
E_A = \int \frac{\left|\phi_A(i,r)\right|^2 Z_A}{r_{iA}} d^3\tau_i \quad \text{and} \quad E_B = \int \frac{\left|\phi_B(i,r-d_1)\right|^2 Z_B}{r_{iB}} d^3\tau_i \tag{S7}
$$

are the atomic terms, describing the core–electron interaction inside an atom,

$$
\Gamma_{Ba} = \int \frac{\left|\phi_A(i,r)\right|^2 Z_B}{r_{iB}} d^3\tau_i \quad \text{and} \quad \Gamma_{Ab} = \int \frac{\left|\phi_B(i,r-d_1)\right|^2 Z_A}{r_{iA}} d^3\tau_i \tag{S8}
$$

describe the core–electron interaction between atoms,

$$
\Gamma_{AB} = \int \phi_A(i,r) \left( \frac{Z_A}{r_{iA}} + \frac{Z_B}{r_{iB}} \right) \phi_B(i,r-d_1)\, d^3\tau_i \tag{S9}
$$

is the intra-cell resonance term, and

$$
\Gamma_{AB}^* = \int \phi_A(r) \left( \frac{Z_A}{r_{iA}} + \frac{Z_B}{r_{iB}+d} \right) \phi_B(i,r-d_1+d)\, d^3\tau_i \tag{S10}
$$

is the inter-cell resonance term.

Similarly, we have

$$
\begin{aligned}
&\left\langle \Psi_k \left| -\frac{Z_A}{r_{Aj}} - \frac{Z_B}{r_{Bj}} \right| \Psi_k \right\rangle \\
=& - c_{A,k}^2 \left(E_A + \Gamma_{Ba}\right) - c_{B,k}^2 \left(E_B + \Gamma_{Ab}\right) - 2c_{A,k}c_{B,k}\Gamma_{AB} - 2c_{A,k}c_{B,k} \cos k \Gamma_{AB}^*
\end{aligned}
\tag{S11}
$$

The electron–electron interaction

$$\begin{aligned}
&\left\langle \Psi_k \left| \frac{1}{r_{ij}} \right| \Psi_k \right\rangle \\
&= c_{A,k}^4 \int\int \frac{|\phi_A(i,r)|^2 |\phi_A(j,r)|^2}{r_{ij}} d^3\tau_i d^3\tau_j \\
&+ c_{B,k}^4 \int\int \frac{|\phi_B(i,r-d_1)|^2 |\phi_B(j,r-d_1)|^2}{r_{ij}} d^3\tau_i d^3\tau_j \\
&+ 2c_{A,k}^2 c_{B,k}^2 \int\int \frac{|\phi_A(i,r)|^2 |\phi_B(j,r-d_1)|^2}{r_{ij}} d^3\tau_i d^3\tau_j \\
&+ 2c_{A,k}^2 c_{B,k}^2 \mathrm{cos}k \int\int \frac{|\phi_A(i,r)|^2 |\phi_B(j,r-d_1+d)|^2}{r_{ij}} d^3\tau_i d^3\tau_j \\
&= c_{A,k}^4 \Gamma_{aa} + c_{B,k}^4 \Gamma_{bb} + 2c_{A,k}^2 c_{B,k}^2 \Gamma_{ab} + 2c_{A,k}^2 c_{B,k}^2 \mathrm{cos}k \Gamma_{ab}^*
\end{aligned} \tag{S12}$$

Here,

$$\Gamma_{aa} = c_{A,k}^4 \int\int \frac{|\phi_A(i,r)|^2 |\phi_A(j,r)|^2}{r_{ij}} d^3\tau_i d^3\tau_j \tag{S13}$$

and

$$\Gamma_{bb} = c_{B,k}^4 \int\int \frac{|\phi_B(i,r-d_1)|^2 |\phi_B(j,r-d_1)|^2}{r_{ij}} d^3\tau_i d^3\tau_j \tag{S14}$$

are also atomic terms, describing the on site Coulomb repulsions.

$$\Gamma_{ab} = c_{A,k}^2 c_{B,k}^2 \int\int \frac{|\phi_A(i,r)|^2 |\phi_B(j,r-d_1)|^2}{r_{ij}} d^3\tau_i d^3\tau_j \tag{S15}$$

describes the Coulomb repulsion between two electrons belong to the two atomic orbitals in a unit cell.

$$\Gamma_{ab}^* = c_{A,k}^2 c_{B,k}^2 \mathrm{cos}k \int\int \frac{|\phi_A(i,r)|^2 |\phi_B(j,r-d_1+d)|^2}{r_{ij}} d^3\tau_i d^3\tau_j \tag{S16}$$

describes the Coulomb repulsion between two electrons belong to the two atomic orbitals in neighboring unit cells.

Summarizing the equations S5, S6, S11, and S12, we have

$$\begin{aligned}
E_k &= 2\left(c_{A,k}^2 K_A + c_{B,k}^2 K_B\right) - 2c_{A,k}^2 \left(E_A + \Gamma_{Ba}\right) - 2c_{B,k}^2 \left(E_B + \Gamma_{Ab}\right) \\
&- 4c_{A,k} c_{B,k} \left(\Gamma_{AB} + \cos k \Gamma_{AB}^*\right) + c_{A,k}^4 \Gamma_{aa} + c_{B,k}^4 \Gamma_{bb} + 2c_{A,k}^2 c_{B,k}^2 \left(\Gamma_{ab} + \cos k \Gamma_{ab}^*\right)
\end{aligned} \tag{S17}$$

## V. SCHEMATIC ILLUSTRATIONS OF CHARGE REDISTRIBUTION UNDER A TENSILE STRAIN

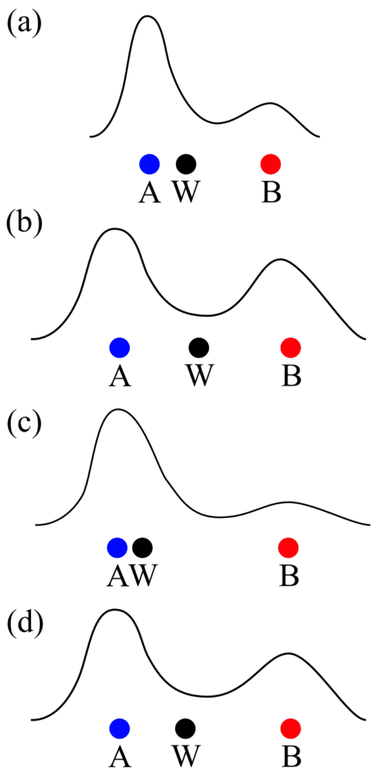


FIG. S2. Schematic plots showing the (a) charge distribution at the unstrained condition, (b) charge redistribution induced by the Coulombic term $\Gamma_{ab}$, in which $\beta$ increases under a tensile strain; (c) charge redistribution induced by the resonance term $\Gamma_{AB}$ in which $\beta$ decreases under a tensile strain; and (d) overall charge redistribution, in which $\beta$ increases under a tensile strain. Here, $A$, $B$, and $W$ represents the positions of the anion, cation, and Wannier center respectively. $\beta = r_w/d_1$, where $r_w$ is the distance between the Wannier center and the position of cation and $d_1$ is the bond length.

## VI. DERIVATION OF EQUATION (9)

In this section, we present detailed derivation of equation (9) in the main text. Fig. S3 shows a schematic plot of a low–dimensional material. The shaded area represents the molecular layer. $c$ is the height of the cell, and $t$ is the thickness of the molecular layer. For the optimized structure, we have $c = c_0$ and $t = t_0$. The ratio of a molecular–layer thickness to the lattice of the cell is $R = t/c$. $h$ represents the distance between the position of an atom and the bottom of the molecular layer. Therefore, the atomic fractional coordinate in the layer scale is $u = h/t$, and the strain of the molecular layer $s = t/t_0 - 1$. The atomic fractional coordinate in the cell scale is $U = h/c$, and the the strain of the cell $S = c/c_0 - 1$. Table S2 summarizes the expressions and descriptions of all these physical quantities.

The change of fractional coordinate inside a molecular layer with the molecular–layer strain is

$$u_s = \frac{\partial u}{\partial s} = \left[\frac{\partial\left(\frac{h}{t}\right)}{\partial\left(\frac{t}{t_0}\right)}\right]\Bigg|_{t=t_0} = \left[t_0\frac{\partial\left(\frac{h}{t}\right)}{\partial t}\right]\Bigg|_{t=t_0} = \left[\frac{t_0}{t}\frac{\partial h}{\partial t} - \frac{t_0 h}{t^2}\right]\Bigg|_{t=t_0} = \frac{\partial h}{\partial t} - \frac{h}{t} \tag{S18}$$

Following similar procedures, we have

$$R_S = \frac{\partial R}{\partial S} = \left[\frac{\partial\left(\frac{t}{c}\right)}{\partial\left(\frac{c}{c_0}\right)}\right]\Bigg|_{c=c_0} = \left[c_0\frac{\partial\left(\frac{t}{c}\right)}{\partial c}\right]\Bigg|_{c=c_0} = \left[\frac{c_0}{c}\frac{\partial t}{\partial c} - \frac{c_0 t}{c^2}\right]\Bigg|_{c=c_0} = \frac{\partial t}{\partial c} - \frac{t}{c}, \tag{S19}$$

and

$$U_S = \frac{\partial U}{\partial S} = \left[\frac{\partial\left(\frac{h}{c}\right)}{\partial\left(\frac{c}{c_0}\right)}\right]\Bigg|_{c=c_0} = \left[c_0\frac{\partial\left(\frac{h}{c}\right)}{\partial c}\right]\Bigg|_{c=c_0} = \left[\frac{c_0}{c}\frac{\partial t}{\partial c} - \frac{c_0 h}{c^2}\right]\Bigg|_{c=c_0} = \frac{\partial h}{\partial c} - \frac{h}{c}. \tag{S20}$$

From the equations (S9) and (S10), we have

$$\frac{\partial h}{\partial t} = u_s + \frac{h}{t} \tag{S21}$$

$$\frac{\partial t}{\partial c} = R_S + \frac{t}{c} \tag{S22}$$

Substitute the equations (S12) and (S13) into the equation (S11), we have

$$\begin{aligned} U_S &= \frac{\partial h}{\partial c} - \frac{h}{c} = \frac{\partial h}{\partial t}\frac{\partial t}{\partial c} - \frac{h}{c} \\ &= \left(u_s + \frac{h}{t}\right)\left(R_S + \frac{t}{c}\right) - \frac{h}{c} = u_s R_S + \frac{h}{t}R_S + u_s\frac{t}{c} \\ &= u_s R_S + u R_S + u_s R = \left(R_S + R\right)u_s + R_S u \end{aligned} \tag{S23}$$

| Physical quantity | Description | Expression |
|---|---|---|
| $U$ | fractional coordinates in the supercell scale | $U = h/c$ |
| $u$ | fractional coordinates in the molecular–layer scale | $u = h/t$ |
| $S$ | strain in the supercell scale | $S = c/c_0 - 1$ |
| $s$ | strain in the molecular–layer scale | $s = t/t_0 - 1$ |
| $U_S$ | change of $U$ with $S$ | $U_S = \partial U/\partial S$ |
| $u_s$ | change of $u$ with $s$ | $u_s = \partial u/\partial s$ |
| $R$ | fraction of a molecular layer in the supercell | $R = t/c$ |
| $R_S$ | change of $R$ with $S$ | $R_S = \partial R/\partial S$ |

TABLE S2. Descriptions and expressions of the physical quantities involved in the derivations.

We would also like to point out that $U_S$ is usually much smaller that $u_s$, since

$$R_S = \frac{\partial R}{\partial S} < 0 \quad \text{and} \quad R = \frac{t}{c} < 1. \tag{S24}$$

Besides, $R = 1$ means that the molecular layer occupies the entire cell, which corresponds to a three–dimensional material. For this case, we have $R_S = \partial R/\partial S = 0$, and

$$U_S = (R_S + R)\, u_s + R_S u = u_s. \tag{S25}$$

Equation (9) is also the equation bridging the piezoelectric responses in low–dimensional piezoelectrics and conventional three–dimensional piezoelectrics.

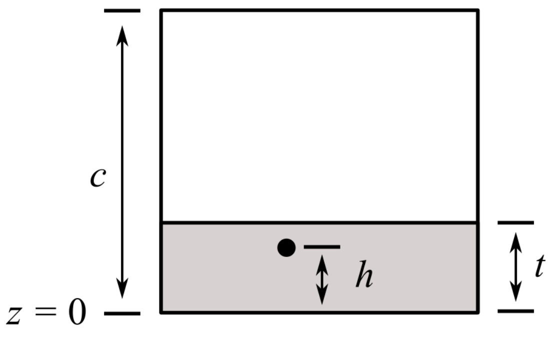


FIG. S3. Schematic plot of a low–dimensional material. The molecular layer region is shaded with the grey color. The height of the cell is $c$, and the thickness of the molecular layer is $t$.

[S1] P. Giannozzi, S. Baroni, N. Bonini, M. Calandra, *et al.*, J. Phys.: Condens. Matter **21**, 395502 (2009).

[S2] http://opium.sourceforge.net.

[S3] J. P. Perdew, K. Burke, and M. Ernzerhof, Phys. Rev. Lett. **77**, 3865 (1996).

[S4] H. J. Monkhorst and J. D. Pack, Phys. Rev. B **13**, 5188 (1976).

[S5] S. Grimme, J. Comput. Chem. **27**, 1787 (2006).

[S6] V. Barone, M. Casarin, D. Forrer, M. Pavone, M. Sambi, and A. Vittadini, J. Comput. Chem. **30**, 934 (2009).

[S7] R. D. King-Smith and D. Vanderbilt, Phys. Rev. B **47**, 1651 (1993).

[S8] F. Bernardini, V. Fiorentini, and D. Vanderbilt, Phys. Rev. B **56**, R10024 (1997).

[S9] L. Bellaiche and D. Vanderbilt, Phys. Rev. B **61**, 7877 (2000).

[S10] G. Sághi-Szabó, R. E. Cohen, and H. Krakauer, Phys. Rev. B **59**, 12771 (1999).

[S11] A. Dal Corso, M. Posternak, R. Resta, and A. Baldereschi, Phys. Rev. B **50**, 10715 (1994).

[S12] F. Tasnadi, B. Alling, C. Höglund, G. Wingqvist, J. Birch, L. Hultman, and I. A. Abrikosov, Phys. Rev. Lett. **104**, 137601 (2010).

[S13] S. Liu and R. Cohen, Phys. Rev. Lett. **119**, 207601 (2017).

[S14] G. Klopman, J. Am. Chem. Soc. **86**, 4550 (1964).
